# Supplementary material for: ML-SemReg: Boosting Point Cloud Registration with Multi-level Semantic Consistency
Source: arXiv:2407.09862 source file (2024-07-13)
Supplement: Supplementary file 1 [file 04_reg_compare.pdf]

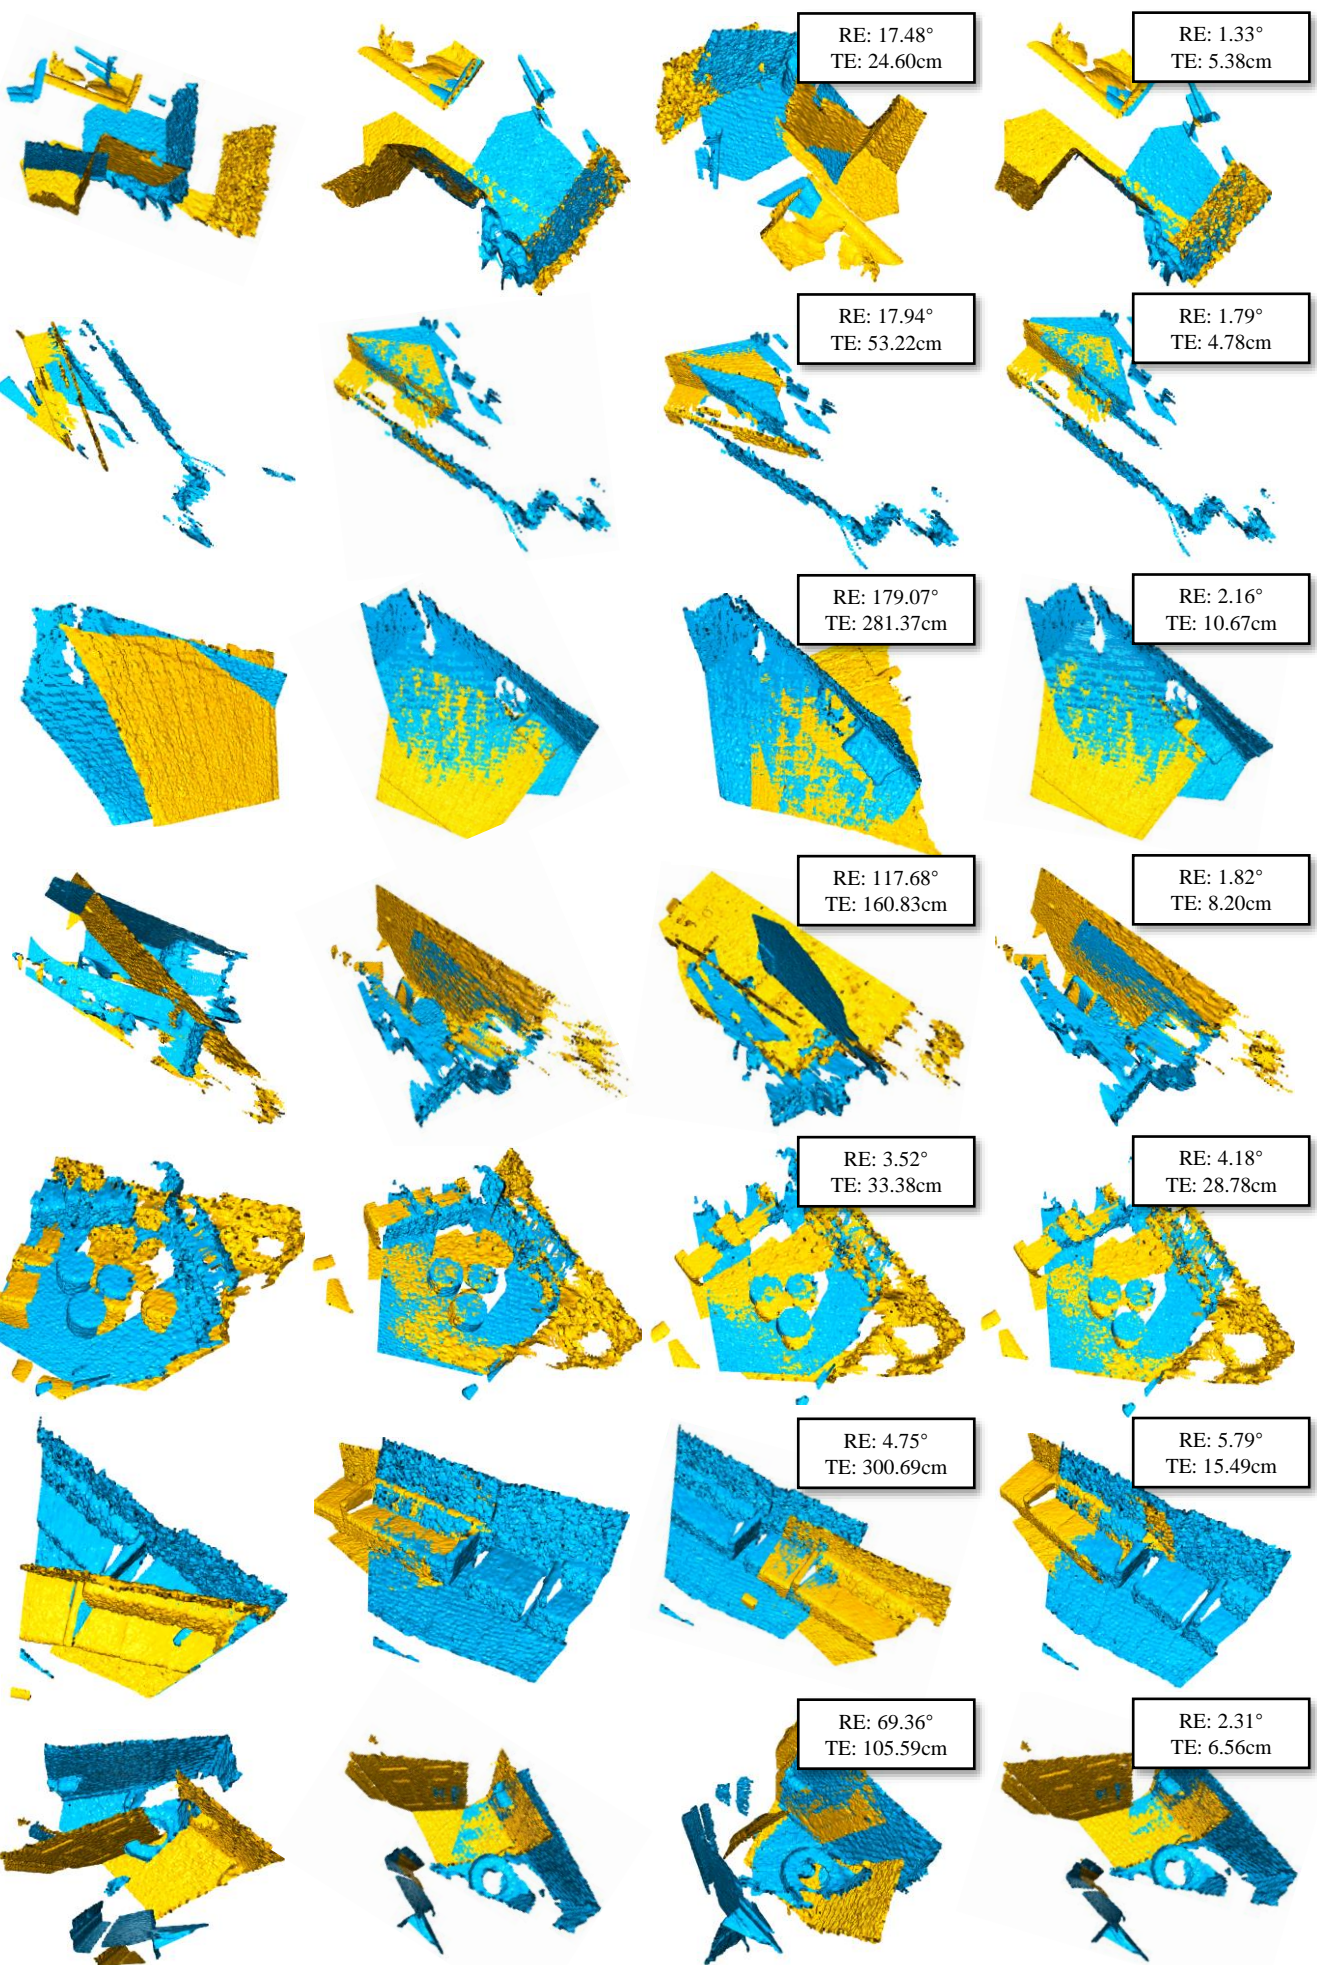

(a) Input

(b) Ground truth

(c) SC2PCR

(d) SC2PCR+Ours



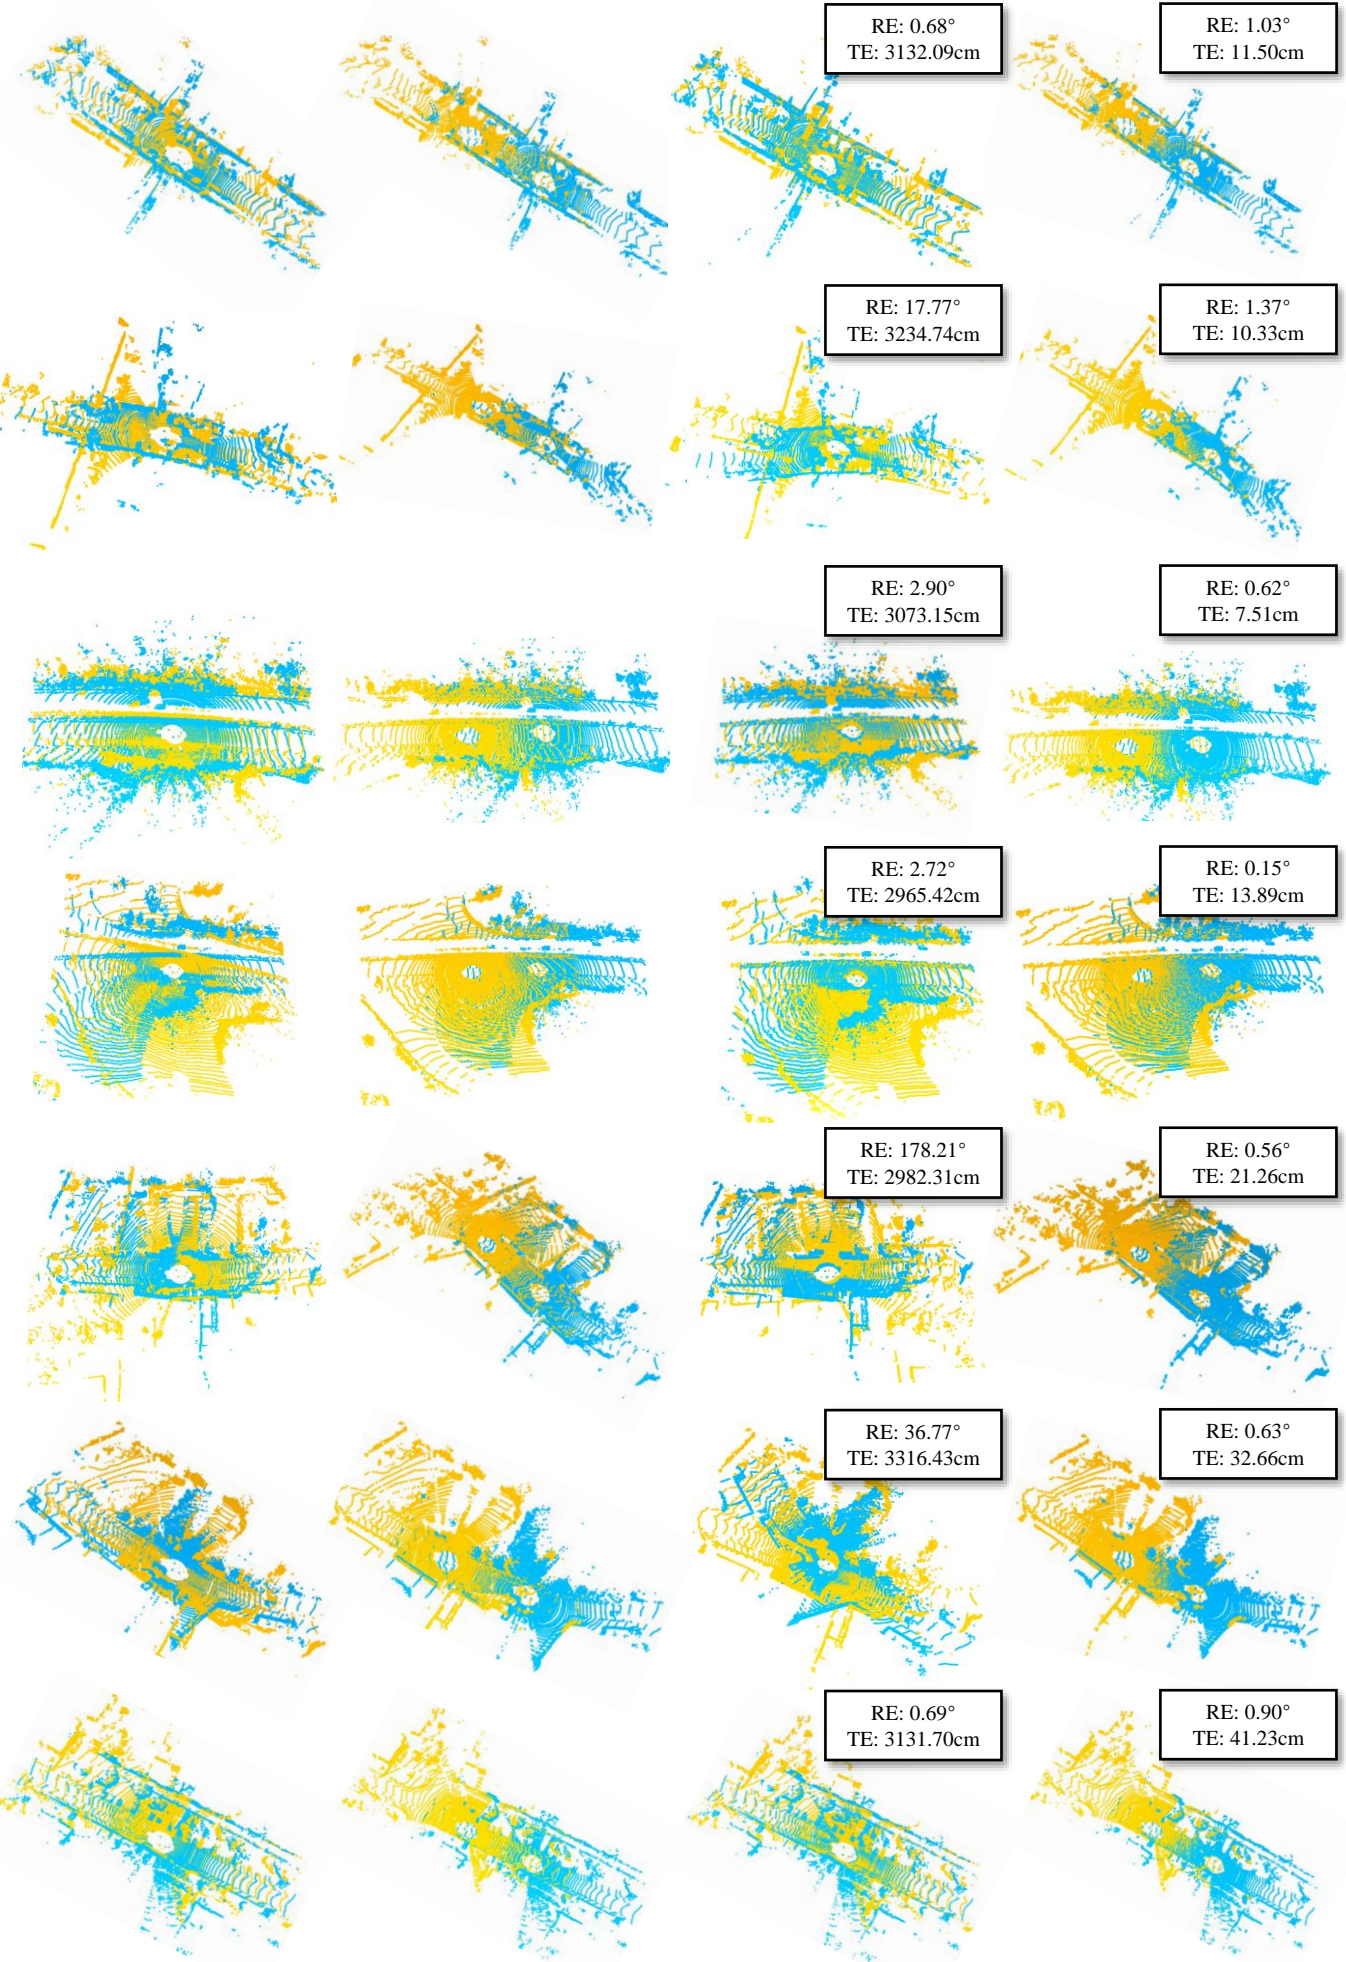

(a) Input

(b) Ground truth

(c) SC2PCR

(d) SC2PCR+Ours
